# Supplementary material for: The Reality of the Situation: A Survey of Situated Analytics
Source: arXiv:2310.10015 source file (2023-10-16)
Supplement: Supplementary file 1 [file appendices.tex]

\newpage
\setcounter{page}{1}
\appendix

\begin{center}
  \huge{Supplemental Material: Sensemaking In Situ}
\end{center}

\section{Classification: Keshif Browser}

We have made our technique classification (Section~\ref{sec:design-space}) publicly (and anonymously) available in a Keshif~\cite{yalcin18keshif} browser: \url{https://explore.keshif.me/5681640172945408/5696764296298496/Situated_visualization}
